# Supplementary material for: Remote Sensing Change Detection via Weak Temporal Supervision
Source: arXiv:2601.02126 source file (2026-11-10)
Supplement: Supplementary file 1 [file main_table_FPR.tex]

\makeatletter
\global\let\oriCT@@do@color\CT@@do@color

\begin{table*}[t!]
  
  \caption{\textbf{Comparison with baselines.} Similar to the table from the main paper but with the false positive rate reported for all methods. Best score for each training data source is highlighted in bold, and the second best score is underlined.}
  \vspace{-2mm}
  \centering  
  \resizebox{\linewidth}{!}{
  \begin{tabular}{ccccc *{2}{wc{\mylen}}ccccccccccc}
    \toprule
    \multirow{4}{*}{\rot[70]{Data source}} & \multirow{4}{*}{Model} & \multirow{4}{*}{\shortstack{Dataset\\extension}} &&&&&&&&&&&&&&&\\
    & & & \multicolumn{6}{c}{In-domain} & \multicolumn{9}{c}{Out-of-Domain}\\
    \cmidrule(lr){4-9}\cmidrule(lr){10-18}
    & & & \multicolumn{3}{c}{b-FLAIR-test} & \multicolumn{3}{c}{b-FLAIR-spot-test} & \multicolumn{3}{c}{LEVIR-CD} & \multicolumn{3}{c}{WHU-CD} & \multicolumn{3}{c}{S2Looking}\\
    \cmidrule(lr){4-6}\cmidrule(lr){7-9}\cmidrule(lr){10-12}\cmidrule(lr){13-15}\cmidrule(lr){16-18}
    & & & $F1\uparrow$ & $IoU\uparrow$ & $FPR\downarrow$ & $F1\uparrow$ & $IoU\uparrow$ & $FPR\downarrow$ & $F1\uparrow$ & $IoU\uparrow$ & $FPR\downarrow$ & $F1\uparrow$ & $IoU\uparrow$ & $FPR\downarrow$ & $F1\uparrow$ & $IoU\uparrow$ & $FPR\downarrow$ \\
    \midrule
    \multirow{5}{*}{\rot[90]{FLAIR}} 
    & UNet      &   ---   & 62.6 & 45.5 & 3.09 & --- & --- & --- & 31.9 & 19.0 & 2.11 & 62.0 & 44.9 & 5.00 & 12.1 & 6.5 & 2.21\\
    & UNet      & b-FLAIR & 65.2 & 48.3 & 2.69 & --- & --- & --- & 35.3 & 21.4 & \underline{2.10} & 65.2 & 48.3 & 4.37 & 12.5 & 6.7 & 1.34\\
    & Dual UNet & FSC-180k~\cite{benidir2025change} & \textbf{83.1} & \textbf{71.1} & \underline{0.73} & --- & --- & --- & \textbf{49}$^\dagger$ & \textbf{33}$^\dagger$ & --- & 63.3 & 46.3 & 3.66 & 4$^\dagger$ & 2$^\dagger$ & ---\\
    & Dual UNet &   ---   & 75.9 & 61.1 & 1.49 & --- & --- & --- & \underline{37.5} & \underline{23.1} & 2.64 & \underline{70.6} & \underline{54.5} & \underline{3.32} & \textbf{13.7} & \textbf{7.4} & \underline{0.72}\\
    \rowcolor{blue!10} \global\let\CT@@do@color\relax & \global\let\CT@@do@color\oriCT@@do@color Dual UNet & b-FLAIR & \underline{79.0} & \underline{65.3} & \textbf{0.35} & --- & --- & --- & 17.8 & 9.3 & \textbf{0.30} & \textbf{77.3} & \textbf{63.0} & \textbf{0.77} & \underline{13.6} & \underline{7.3} & \textbf{0.58} \\
    \midrule
    \addlinespace[3mm]
    \multirow{4}{*}{\rot[90]{~~FLAIR-spot}}
    & UNet      &      ---     & --- & --- & --- & 24.1 & 13.7 & 6.78 & 3.0 & 1.5 & \underline{0.49} & 15.2 & 8.2 & 6.14 & 0.4 & 0.2 & \underline{0.06}\\
    & UNet      & b-FLAIR-spot & --- & --- & --- & \underline{25.0} & \underline{14.3} & 6.02 & \underline{19.5} & \underline{10.8} & 13.3 & \underline{28.6} & \underline{16.7} & 10.1 & \underline{1.9} & \underline{1.0} & 0.32 \\
    & Dual UNet &      ---     & --- & --- & --- & \textbf{29.2} & \textbf{17.1} & \underline{4.83} & 0.7 & 0.4 & \textbf{0.12} & 5.2 & 2.7 & \textbf{1.12} & 0.1 & 0 & \textbf{0.02}\\
    \rowcolor{blue!10} \global\let\CT@@do@color\relax & \global\let\CT@@do@color\oriCT@@do@color Dual UNet & b-FLAIR-spot & --- & --- & --- & 22.9 & 12.9 & \textbf{0.31} & \textbf{34.1} & \textbf{20.6} & 4.04 & \textbf{49.3} & \textbf{32.7} & \underline{3.42} & \textbf{7.1} & \textbf{3.7} & 1.57 \\
    \addlinespace[3mm]
    \midrule
    \multirow{4}{*}{\rot[90]{IAILD}}
    & UNet      &   ---   & --- & --- & --- & --- & --- & --- & \underline{53.1} & \underline{36.2} & 3.0 &            42.6  &            27.1  & 10.1 &             4.6  &            2.4  & 19.7\\
    & UNet      & b-IAILD & --- & --- & --- & --- & --- & --- &            44.9  &            28.9  & \underline{1.8} &            44.5  &            28.6  & 8.1 &  \underline{7.9} & \underline{4.1} & \underline{9.7}\\
    & Dual UNet &   ---   & --- & --- & --- & --- & --- & --- &    \textbf{54.7} &    \textbf{37.6} & 3.3 & \underline{53.7} & \underline{36.7} & \underline{7.1} &             6.1  &            3.1  & 12.7\\
    \rowcolor{blue!10} \global\let\CT@@do@color\relax & \global\let\CT@@do@color\oriCT@@do@color Dual UNet & b-IAILD & --- & --- & --- & --- & --- & --- &            35.9  &            21.9  & \textbf{0.3} &    \textbf{63.3} &    \textbf{46.3} & \textbf{1.9} &    \textbf{17.6} &    \textbf{9.6} & \textbf{2.4} \\
    
    \midrule
    
    & Dual UNet & SyntheWorld~\cite{song2024syntheworld} & --- & --- & --- & --- & --- & --- & 25$^\dagger$ & 13$^\dagger$ & --- & 25.1 & 14.3 & 11.2 & 0$^\dagger$ & 0$^\dagger$ & --- \\
    \bottomrule
  \end{tabular}}
  \vspace{-.5em}
  \label{tab:comparison_results_supp_mat}
\end{table*}
